# Supplementary material for: All-relevant feature selection using multidimensional filters with exhaustive search
Source: arXiv:1705.05756 source file (2017-05-16)
Supplement: Supplementary file 1 [file appendix_c.tex]

\section{Discretisation}

%\section{The method of discretisation}
\subsection{Split into equipotent categories}
\label{dyskretyz}
The simplest idea of discretization of a continuous variable is a standard histogram-building procedure: the range of values of the variable is split into a number of equal intervals, corresponding to the categories of the discretized variable. However, such a procedure often produces categories, that contain very few (or zero) objects in the analyzed dataset. This causes sparsity of the contingency table, which interferes the distribution of the tested quantities. 

Therefore, the important purpose of the discretization procedure is to avoid the risk of sparsity of the contingency tables. The risk is minimized, if each category of the variable contains the same number of objects. So, our approach to the discretization is to split the range of the variable into categories, that contain numbers of objects as close to each other as possible. Of course, the identical values of the variable should correspond to the same category (see Fig.~\ref{dyskr1}). 

\subsection{Randomly shifted splits}
However, the discretization always causes lost of information about the variable. It could happen, that the existing dependence between the variables would not be detectable due to the unfortunate discretization choice (see Fig.~\ref{dyskr2}). Discretization into more categories reduces the risk, but makes the calculations much slower. Surprisingly, performing the analysis several times for discretizations with randomly shifted splits can take less time.

\begin{figure}
\centering
\begin{tabular}{ll}
{\bf a)}&{\bf b)}\\
\includegraphics[width=0.4\textwidth]{dyskr1.pdf}&
\includegraphics[width=0.4\textwidth]{dyskr2.pdf}\\
\end{tabular}
\caption{
a) The discretization into the equal intervals can produce very few objects in some categories.
b) The discretization into equipotent categories minimizes the risk of sparsity of the contingency tables.
}
\label{dyskr1}
\end{figure}

In this case, we should take the minimum $p$-value for each variable obtained over all the discretizations and the $k$-tuples. This is still the extreme value statistics, so $p_{min}$ follows the exponential distribution, however, the $\gamma$ parameter will be smaller. That means, that more tests for each variable increases the probability of false positive results. Therefore, the number of discretizations shouldn't be too big, even if the number of variables is small enough to maintain the reasonable time of calculations.
